# Supplementary material for: s+if pairing in Ising superconductors
Source: arXiv:1902.02577 source file (2019-02-07)
Supplement: Supplementary file 1 [file IsingGL_suppl.pdf]

# Supplemental Material: $s+if$ pairing in Ising superconductors

David Möckli and Maxim Khodas
*The Racah Institute of Physics, The Hebrew University of Jerusalem, Jerusalem 9190401, Israel*
(Dated: February 7, 2019)

Here we discuss the technical details, which are inessential for the main text's conclusions. We derive the free energy from the Hamiltonian, evaluate the momentum and Matsubara sums, describe limited and protected order parameters, discuss the role of the $A_1'$ triplet channel, show the quasi-particle dispersion and list the animations found in the supplemental material section.

## I. DERIVATION OF THE FREE ENERGY

The derivation procedure is standard and can be found in many books [1]. The mean-field Hamiltonian is

$$H = \sum_{\mathbf{k},s} \xi_{\mathbf{k}} c^\dagger_{\mathbf{k}s} c_{\mathbf{k}s} + \sum_{\mathbf{k},ss'} (\boldsymbol{\gamma}_{\mathbf{k}} - \mathbf{B}) \cdot \boldsymbol{\sigma}_{ss'} c^\dagger_{\mathbf{k}s} c_{\mathbf{k}s'} + \frac{1}{2} \sum_{\mathbf{k},s_1 s_2} \left[ \Delta_{s_1 s_2}(\mathbf{k}) c^\dagger_{\mathbf{k}s_1} c^\dagger_{-\mathbf{k},s_2} + \Delta^*_{s_1 s_2}(\mathbf{k}) c_{-\mathbf{k},s_2} c_{\mathbf{k}s_1} \right]$$
$$- \frac{1}{2} \sum_{\mathbf{k},\mathbf{k}'} \sum_{s_i, s_i'} \Delta^*_{s_1' s_2'}(\mathbf{k}') V^{-1}_{s_1' s_2', s_1 s_2}(\mathbf{k}', \mathbf{k}) \Delta_{s_1 s_2}(\mathbf{k}), \quad \text{with} \quad \Delta_{s_1 s_2}(\mathbf{k}) = \sum_{\mathbf{k}', s_1' s_2'} V_{s_1 s_2, s_1' s_2'}(\mathbf{k}, \mathbf{k}') \langle c_{-\mathbf{k}' s_2'} c_{\mathbf{k}' s_1'} \rangle. \tag{1}$$

Note that the interaction amplitude satisfies, $V_{s_1 s_2, s_1' s_2'}(\mathbf{k}, \mathbf{k}') = V^*_{s_1' s_2', s_1 s_2}(\mathbf{k}', \mathbf{k})$. Considering the three indices as a single label, $j = (s_1, s_2, \mathbf{k})$ the above relation implies Hermiticity, $V_{j,j'} = V^*_{j',j}$. We assume the $V_{j,j'}$ matrix has an inverse which satisfies

$$\sum_{s_1', s_2', \mathbf{k}'} V_{s_1 s_2, s_1' s_2'}(\mathbf{k}, \mathbf{k}') V^{-1}_{s_1' s_2', s_1'' s_2''}(\mathbf{k}', \mathbf{k}'') = \delta_{s_1, s_1''} \delta_{s_2, s_2''} \delta_{\mathbf{k}, \mathbf{k}''}\,, \tag{2}$$

The inverse matrix, $V^{-1}$ is Hermitian as well. This ensures that the last term of the mean field Hamiltonian, Eq. (1) is real valued as expected.

We write the creation and annihilation operators as Grassmann variables $c^\dagger \to \bar{c}$, such that the action reads $S = \int_0^\beta \mathrm{d}\tau \left( \bar{c}_{\mathbf{k}s} \partial_\tau c_{\mathbf{k}s} + H \right)$, where $\tau$ is imaginary time and $\beta = 1/T$. We Fourier transform from imaginary time $\tau$ to Mastsubara frequencies $\omega_n = (2n+1)\pi/\beta$ as $c_{\mathbf{k}s}(\tau) = \beta^{-1/2} \sum_n \psi_{\mathbf{k}ns} e^{-i\omega_n \tau}$. Then

$$S = \frac{1}{2} \sum_{\mathbf{k},\omega_n} \bar{\mathbf{\Phi}}^{\mathrm{T}}_{\mathbf{k}n} \left[ -\mathcal{G}_0^{-1}(\mathbf{k}, \omega_n) + \mathbf{\Delta}(\mathbf{k}) \right] \mathbf{\Phi}_{\mathbf{k}n} - \frac{\beta}{2} \sum_{\mathbf{k},\mathbf{k}'} \sum_{s_i, s_i'} \Delta^*_{s_1' s_2'}(\mathbf{k}') V^{-1}_{s_1' s_2', s_1 s_2}(\mathbf{k}', \mathbf{k}) \Delta_{s_1 s_2}(\mathbf{k}), \tag{3}$$

where $\mathbf{\Phi}_{\mathbf{k}n} = \left( \psi_{\mathbf{k}n\uparrow}, \psi_{\mathbf{k}n\downarrow}, \bar{\psi}_{-\mathbf{k},-n\uparrow}, \bar{\psi}_{-\mathbf{k},-n\downarrow} \right)^{\mathrm{T}}$, and the $4 \times 4$ matrices $\mathcal{G}_0^{-1}(\mathbf{k}, \omega_n)$ and $\mathbf{\Delta}(\mathbf{k})$ can be written in terms of more familiar $2 \times 2$ matrices as

$$\mathcal{G}_0^{-1}(\mathbf{k}, \omega_n) = \begin{bmatrix} G^{-1}(\mathbf{k}, \omega_n) & 0 \\ 0 & -G^{-1,\mathrm{T}}(-\mathbf{k}, -\omega_n) \end{bmatrix}, \qquad \mathbf{\Delta}(\mathbf{k}) = \begin{bmatrix} 0 & \Delta_{\mathbf{k}} \\ \Delta^\dagger_{\mathbf{k}} & 0 \end{bmatrix}, \tag{4}$$

with the Green function $G(\mathbf{k}, \omega_n) = G_+(\mathbf{k}, \omega_n) \sigma_0 + G_-(\mathbf{k}, \omega_n)\, \mathfrak{g}_{\mathbf{k}} \cdot \boldsymbol{\sigma}$ and $\Delta_{\mathbf{k}} = (\psi_{\mathbf{k}} \sigma_0 + \mathbf{d}_{\mathbf{k}} \cdot \boldsymbol{\sigma}) i\sigma_y$, (see the main text for explicit expressions for the Green functions). We can now calculate the partition function

$$Z = \int \mathcal{D}\bar{\mathbf{\Phi}}_{\mathbf{k}n} \mathcal{D}\mathbf{\Phi}_{\mathbf{k}n}\, e^{-S} = e^{-S_{\mathrm{eff}}}, \tag{5}$$

to obtain the effective action $S_{\mathrm{eff}}$, or alternatively, the free energy $F = S_{\mathrm{eff}}/\beta$, which reads

$$F = -\frac{1}{2} \sum_{\mathbf{k},\mathbf{k}'} \sum_{s_i, s_i'} \Delta^*_{s_1' s_2'}(\mathbf{k}') V^{-1}_{s_1' s_2', s_1 s_2}(\mathbf{k}', \mathbf{k}) \Delta_{s_1 s_2}(\mathbf{k}) - \frac{1}{\beta} \sum_{\mathbf{k},\omega_n} \mathrm{tr}\, \ln \frac{\beta}{2} \left( -\mathcal{G}_0^{-1}(\mathbf{k}, \omega_n) + \mathbf{\Delta}(\mathbf{k}) \right). \tag{6}$$

We can expand the logarithm in the second term and write the free energy as

$$F = -\frac{1}{2} \sum_{\mathbf{k},\mathbf{k}'} \sum_{s_i, s_i'} \Delta^*_{s_1' s_2'}(\mathbf{k}') V^{-1}_{s_1' s_2', s_1 s_2}(\mathbf{k}', \mathbf{k}) \Delta_{s_1 s_2}(\mathbf{k}) + \frac{1}{\beta} \sum_{\mathbf{k},\omega_n} \sum_{l=1}^{\infty} \frac{(-2)^l}{2l} \mathrm{tr} \left[ G(\mathbf{k}, \omega_n) \Delta_{\mathbf{k}} G^{\mathrm{T}}(-\mathbf{k}, -\omega_n) \Delta^\dagger_{\mathbf{k}} \right]^l, \tag{7}$$

where we did not include the free energy of the normal state that does not depend on $\Delta_{\mathbf{k}}$.

## II. ENERGY INTEGRALS AND MATSUBARA SUMS

To perform the sum over $\{\mathbf{k},\omega_n\}$ of the Green's function products, it is convenient to rewrite the products as [2]

$$G_\pm(\mathbf{k},\omega_n)G_\pm(-\mathbf{k},-\omega_n)=\frac{1}{4}\sum_{\lambda=\pm}\left[\frac{1}{\omega_n^2+(\xi_\mathbf{k}+\lambda|\gamma_\mathbf{k}|)^2}\pm\frac{1}{(\omega_n+i\lambda|\gamma_\mathbf{k}|)^2+\xi_\mathbf{k}^2}\right]. \tag{8}$$

Using the single density of states $N_0$ approximation for the spin-split bands, the sum over momentas $\mathbf{k}$ can be converted to an integral over energy $\xi$ as $\sum_\mathbf{k}\to N_0\int_0^{2\pi}\frac{\mathrm{d}\varphi}{2\pi}\int_{-\epsilon_c}^{\epsilon_c}\mathrm{d}\xi$, and we obtain

$$\frac{1}{\beta}\sum_{\omega_n}\int_{-\epsilon_c}^{\epsilon_c}\mathrm{d}\xi\,G_+(\mathbf{k},\omega_n)G_+(-\mathbf{k},-\omega_n)=\ln\left(\frac{2e^\gamma}{\pi}\frac{\epsilon_c}{T}\right)-\frac{1}{2}\left[\mathrm{Re}\,\psi\left(\frac{1}{2}+i\frac{\sqrt{|\gamma_\mathbf{k}|^2+B^2}}{2\pi T}\right)-\psi\left(\frac{1}{2}\right)\right]; \tag{9}$$

$$\frac{1}{\beta}\sum_{\omega_n}\int_{-\epsilon_c}^{\epsilon_c}\mathrm{d}\xi\,G_-(\mathbf{k},\omega_n)G_-(-\mathbf{k},-\omega_n)=\frac{1}{2}\left[\mathrm{Re}\,\psi\left(\frac{1}{2}+i\frac{\sqrt{|\gamma_\mathbf{k}|^2+B^2}}{2\pi T}\right)-\psi\left(\frac{1}{2}\right)\right]. \tag{10}$$

Integrals involving $G_+G_-$ vanish. The right-hand sides of Eqs. (9,10) still depend on the angle $\varphi_\mathbf{k}$. Instead of performing the angular integrals, a good approximation is to substitute $|\gamma_\mathbf{k}|^2$ by $\int_0^{2\pi}\frac{\mathrm{d}\varphi}{2\pi}|\gamma_\mathbf{k}|^2\equiv\langle|\gamma_\mathbf{k}|^2\rangle_{\mathrm{FS}}=\Delta_{\mathrm{so}}^2$, which allows us to obtain simple analytic and physically transparent results.

The quartic terms involve products of four Green's functions. Although the evaluation is straightforward, the cumbersome task can be avoided with a *Wolfram Mathematica* script.

## III. LIMITED AND PROTECTED ORDER PARAMETERS

It is instructive to write the terms multiplying $G_-(\mathbf{k},\omega_n)G_-(-\mathbf{k},-\omega_n)$ in the trace of Eq. (7) with $l=1$ explicitly to see which order parameters are limited/protected against the Zeeman field and SOC. Simply put, positive contributions to the free energy limit superconductivity, whereas negative terms protect it. The first contribution is

$$\mathfrak{g}_\mathbf{k}\cdot\mathfrak{g}_{-\mathbf{k}}|\psi_\mathbf{k}|^2\to\frac{B^2-\Delta_{\mathrm{so}}^2}{\Delta_{\mathrm{so}}^2+B^2}|\psi_0|^2, \tag{11}$$

which tells us that the Zeeman field limits singlets, and SOC protects them. The second term is

$$(\mathfrak{g}_\mathbf{k}\cdot\mathbf{d}_\mathbf{k})(\mathfrak{g}_{-\mathbf{k}}\cdot\mathbf{d}_\mathbf{k}^*)\to\frac{1}{\Delta_{\mathrm{so}}^2+B^2}\left[|B_x\eta_x+B_y\eta_y|^2-\Delta_{\mathrm{so}}^2|\eta_z|^2\right]. \tag{12}$$

If $(B_x,B_y)=(B,0)$, the first term vanishes with $\eta_x=0$. The second term shows that $\eta_z$ is protected by SOC. The third term is

$$-(\mathfrak{g}_\mathbf{k}\times\mathbf{d}_\mathbf{k})\cdot(\mathfrak{g}_{-\mathbf{k}}\times\mathbf{d}_\mathbf{k}^*)\to\frac{1}{\Delta_{\mathrm{so}}^2+B^2}\left[\Delta_{\mathrm{so}}^2\left(|\eta_x|^2+|\eta_y|^2\right)-B^2|\eta_z|^2-|B_x\eta_y-B_y\eta_x|^2\right]. \tag{13}$$

A $d$-vectors lying in the plane is limited by SOC in the same way singlets are limited by the Zeeman field. The second terms shows that $\eta_z$ is protected against the Zeeman field. From the last term we see that in-plane $d$-vector components that are orthogonal to the Zeeman field are favourable at finite fields. The last and central term of the paper is

$$2\psi_\mathbf{k}\,\mathfrak{g}_\mathbf{k}\times\mathfrak{g}_{-\mathbf{k}}\cdot\mathrm{Im}\,\mathbf{d}_\mathbf{k}\to\frac{4\psi_0\Delta_{\mathrm{so}}}{\Delta_{\mathrm{so}}^2+B^2}\left(B_y\tilde{\eta}_x-B_x\tilde{\eta}_y\right),\quad\text{where}\quad\tilde{\eta}_y=\mathrm{Im}\,\eta_y, \tag{14}$$

which mixes $A_1'$ singlets with $E''$ triplets and is always favourable at finite Zeeman fields. *Moral of the story: the Zeeman field limits $\psi_0$, SOC limits $\{\eta_x,\eta_y\}$, but they are induced by field, and $\eta_z$ is protected against both Zeeman fields and SOC.*

## IV. THE FREE ENERGY INCLUDING THE $A_1'$ TRIPLET CHANNEL

The free energy including the $\eta_z$ triplets with critical temperature $T_{\rm ctz}$ and $B_x = B$ ($\eta_x = 0$) reads

$$\frac{1}{2N_0} F_{T,B}[\psi_0, \eta_y, \eta_z] = \alpha_s(T_{\rm cs}, B)\psi_0^2 + \alpha_t(T_{\rm cs}, B)\eta_y^2 + \ln\left(\frac{T}{T_{\rm ctz}}\right)\eta_z^2 + 2\alpha_{st}(B)\psi_0\eta_y$$
$$+ \beta_1(B)\left(B\psi_0 - \Delta_{\rm so}\eta_y\right)^2\left[\left(\Delta_{\rm so}\psi_0 + B\eta_y\right)^2 - \eta_z^2\left(\Delta_{\rm so}^2 + B^2\right)\right]$$
$$+ \beta_2(B)\left(B\psi_0 - \Delta_{\rm so}\eta_y\right)^4 + \beta_3(B)\left[\left(\Delta_{\rm so}\psi_0 + B\eta_y\right)^4 + 6\eta_z^2\left(\Delta_{\rm so}\psi_0 + B\eta_y\right)^2\left(\Delta_{\rm so}^2 + B^2\right) + \eta_z^4\left(\Delta_{\rm so}^2 + B^2\right)^2\right], \quad (15)$$

In the regime $\Delta_{\rm so}/E_{\rm F} \ll 1$, the order parameter $\eta_z$ is decoupled from $\{\psi_0, \eta_y\}$ at the quadratic level and the Zeeman field is the only source of singlet-triplet mixing. However, $\eta_z$ mixes with $\{\psi_0, \eta_y\}$ at the quartic level, which leads to a first-order phase transition between $\eta_z$ and $\{\psi_0, \eta_y\}$ below $T_{\rm ctz}$ at high fields; see Fig. 1d in the main text.

## V. THE QUASI-PARTICLE DISPERSION

We can diagonalize the mean-field Hamiltonian (1) to obtain the quasi-particle dispersions

$$E_{\mathbf{k}\pm}^2 = \xi_{\mathbf{k}}^2 + B^2 + \psi_0^2 + \left(\eta_y^2 + \Delta_{\rm so}^2\right)\hat{\gamma}_{\mathbf{k}}^2 \pm 2\left[\left(B\psi_0 - \Delta_{\rm so}\eta_y\hat{\gamma}_{\mathbf{k}}^2\right)^2 + \xi_{\mathbf{k}}^2\left(B^2 + \Delta_{\rm so}^2\gamma_{\mathbf{k}}^2\right)\right]^{\frac{1}{2}}. \quad (16)$$

We then use the GL solution for $\{\psi_0, \eta_y\}$ as input for Eq. (16) to study the evolution of $E_{\mathbf{k}\pm}(B)$ at a fixed temperature. $E_{\mathbf{k}\pm}$ simplifies on the $M\Gamma$ high symmetry lines, along which $\hat{\gamma}_{\mathbf{k}} = 0$, yielding $|E_{\mathbf{k}\pm}| = |\left(\xi_{\mathbf{k}}^2 + \psi_0^2\right)^{\frac{1}{2}} \pm B|$. This implies that a pair of nodes appear along each $M\Gamma$ line for $B_{\rm n} > \psi_0$. The transition from the fully gapped to the nodal phase is a topological transition [3].

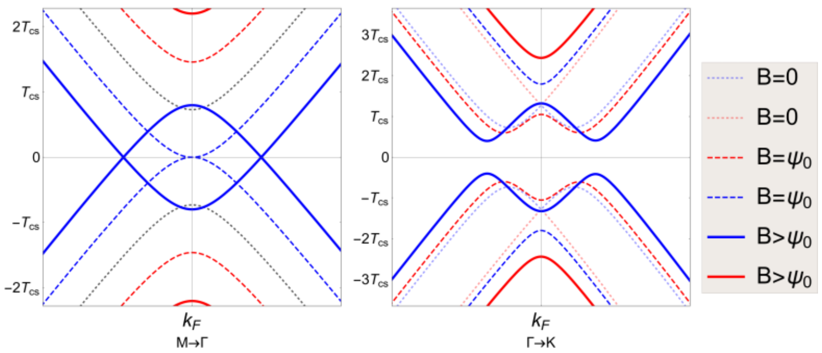


FIG. 1. Quasi-particle dispersions are shown for the $M\Gamma$ (only Zeeman splitting) and $\Gamma K$ (Zeeman and SOC splitting) directions. We used $\xi_{\mathbf{k}} = -(k_x^2 + k_y^2)/2m + \mu$ with $m = 1$, $\mu = 2\pi^2/9m$, $T_{\rm cs} = \mu/100$, $\Delta_{\rm so} = 10T_{\rm cs}$, and $k_{\rm F}^2 = 2m\mu$. See *dispersion120ms.gif* for an animated version.

## VI. ANIMATIONS

The following .gif animations can be found in the *supplemental material* section.

- **dispersion120ms.gif** The evolution of the quasi-particle dispersion with increasing magnetic field at $T = 0.7T_{\rm cs}$ with $T_{\rm ct} = 0.1T_{\rm cs}$. The green point indicates the topological transition. The Zeeman and SOC split bands are shown in red and blue. Whereas the $M\Gamma$ direction is split by the Zeeman field only, the $\Gamma K$ direction is also subjected to SOC.

- **line100ms.gif** Evolution of the normal state to superconducting transition lines for increasing SOC. Here $T_{\rm ct} = 0.05T_{\rm cs}$.

[1] A. Altland and B. D. Simons, "Broken symmetry and collective phenomena," in *Condensed Matter Field Theory* (Cambridge University Press, 2010) pp. 242–359, 2nd ed.
[2] M. Sigrist, in *AIP Conference Proceedings*, Vol. 55 (AIP, 2009) pp. 55–96.
[3] W.-Y. He, B. T. Zhou, J. J. He, N. F. Q. Yuan, T. Zhang, and K. T. Law, Communications Physics **1**, 40 (2018).
